# Supplementary material for: Mapping dust in the giant molecular cloud Orion A
Source: arXiv:2401.12976 source file (2024-01-23)
Supplement: Supplementary file 1 [file appendix_5.tex]

\label{sec:appendix_5}

These two types of extinction data---computed and inferred---are of very different kinds.
In the first case, of direct calculation, extinctions are represented as point observations together with an uncertainty, and we can always decompose them into a signal term and a noise term.
In the second case, of inference, extinctions are represented as probability density functions.
These may may be multimodal and skewed, and may not be decomposed into a signal and an error (Fig.~B2 in the paper by \citealt{anders_photo-astrometric_2019} shows the posterior probability density functions for the extinction of several sources).
When making three-dimensional dust maps of interstellar dust we would like to be able to infer the extinction at an arbitrary point using data of either kind.
